# Supplementary material for: Aerial Shepherds: Enabling Hierarchical Localization in Heterogeneous MAV Swarms
Source: arXiv:2506.08408 source file (2025-06-10)
Supplement: Supplementary file 1 [file Appendix.tex]

\appendices

% \section{Key definitions}\label{A1}
% % In this section, we define several key concepts and summarize main notations and descriptions in Appendix \ref{notation}.

% \subsection{Environmental Description} 
% Let $\Omega$ be a bounded space in $\mathbb{R}^3$ with length, width, and height $L$, $W$, and $H$, respectively, where the heterogeneous MAV swarm operates.
% This swarm comprises a fixed number of BMAVs and AMAVs that operate independently. 
% For simplicity, we assume that both types of MAVs operate at the same altitude in this paper.
% % By increasing the velocity perpendicular to the ground, the swarm can operate in three-dimensional space.

% \subsection{State model of AMAV} 
% The heterogeneous MAV swarm contains $M$ ($M$ \textgreater $1$) AMAVs. The state of each AMAV $A_j$ at time $t$ consists of the location and the motion command.
% The location is denoted as $\boldsymbol{x_{j,t}}=(x_{j,t}^1, x_{j,t}^2, \phi_{j,t})$, where $\phi_{j,t}$ is the orient angle. The distance between two locations is $d_{\chi}$. For motion command, $\boldsymbol{u_{j, t}} = (u_{j,t}, \omega_{j,t})$, where $u_{j,t}$ and $\omega_{j,t}$ are the translational and rotational velocities, respectively.
% The AMAVs estimate their location accurately with advanced sensing capabilities and follow the motion model $\boldsymbol{x_{j, t}} = f(\boldsymbol{x_{j, t-1}}, \boldsymbol{u_{j, t-1}})$, which can be represented as follows:
% \begin{equation}
% \left(\begin{array}{c}
% x_{j,t}^1 \\
% x_{j,t}^2 \\
% \phi_{j,t}
% \end{array}\right) =
% \left(\begin{array}{c}
% x_{j,t-1}^1 \\
% x_{j,t-1}^2 \\
% \phi_{j,t-1}
% \end{array}\right) + \left(\begin{array}{c}
% u_{j,t-1} \cos \left(\phi_{j,t-1}\right) \\
% u_{j,t-1} \sin \left(\phi_{j,t-1}\right) \\
% \omega_{j,t-1}
% \end{array}\right).
% % \vspace{-0.4em}
% \end{equation}

% \subsection{State model of BMAV} 
% The heterogeneous MAV swarm includes $N$ ($N$\textgreater$1$) BMAVs. The state of each BMAV $B_i$ at time $t$ consists of the location and the motion command.
% The location of $B_i$ is $\boldsymbol{y_{i, t}}=(y_{i,t}^1, y_{i,t}^2)$, and its motion command is $\boldsymbol{v_{i, t}} = (v_{i,t}^1, v_{i,t}^2)$.
% $B_i$ follows double integrator dynamics with Gaussian noise represented as follows \cite{purohit2013sugarmap}:
% \begin{equation}
% \begin{gathered}
% \left(\begin{array}{l}
% y_{i, t+\delta}^1 \\
% y_{i, t+\delta}^2
% \end{array}\right)=\left(\begin{array}{l}
% y_{i, t}^1 \\
% y_{i, t}^2
% \end{array}\right)+\delta\left(\begin{array}{l}
% v_{i, t}^1+n_{i, t}^1 \\
% v_{i, t}^2+n_{i, t}^2
% \end{array}\right),\\
% \text{$n_{i, t}^1$ is drawn from $p(n^1)$,} \\
% \text{$n_{i, t}^2$ is drawn from $p(n^2)$,}
% \end{gathered}
% \label{y}
% \end{equation}
% where $n_{i, t}^1$ and $n_{i, t}^2$ are drawn from motion noise models $p(n^1)$ and $p(n^2)$ respectively, $\delta$ ($\delta > 1$) denotes the time interval between two commands.
% $p(n^1)$ and $p(n^2)$ empirically obtained from the testbed are specified as normal distributions with mean $\mu = 0$ and variance $\sigma$, expressed as a percentage of $v_{i, t}^1$ and $v_{i, t}^2$, same as outlined in \cite{chen2020h}.
% % Due to limited onboard capability and the absence of localization infrastructure, the \textit{Resource Allocation System} cannot obtain actual locations and motion commands of the BMAVs.
% The location estimation of $B_i$ is denoted as $\boldsymbol{\widehat{y}_{i, t}}$, and the covariance matrix is denoted as $\Sigma_{i, t}$.
% The noisy motion measurement from $B_i$'s IMU is denoted as $\boldsymbol{\dot{v}_{i, t}}$.


% \subsection{Observation model of AMAV}
% % $A_j$ is equipped with a visual sensor that can generate observations for BMAVs with respect to their actual locations.
% The observation angle of the visual sensor is denoted by $\phi$, and the FoV of $A_j$ at time $t$ is defined as follows,
% \begin{equation}
% \begin{aligned}
% & F_{j, t}=\{(x, y) \mid \\
% & \quad \quad 0<\sqrt{\left(y-x_{j,t}^2\right)^2+\left(x-x_{j,t}^1\right)^2}<r_m \quad \bigcap \\
% & \quad -\frac{\phi}{2}<\arctan\left(\left(y-x_{j,t}^2\right)\left(x-x_{j,t}^1\right)\right)-\phi<\frac{\phi}{2}\}, 
% \end{aligned}
% \label{F_t}
% \end{equation}
% where $r_m$ is the maximum distance that the sensor can observe, which is limited by the observation technique.

% When $B_i$ in the FoV of $A_j$ at time $t$, $A_j$ generates noisy observation $z_{i, j, t}$ for $B_i$, which consists of range $r_{i, j, t}$ and bearing $\alpha_{i, j, t}$  for $B_i$, both $r_{i, j, t}$ and $\alpha_{i, j, t}$ are relative to $A_i$,
% \begin{equation}
% \begin{gathered}
% \begin{aligned}
% z_{i, j, t}
% &=h(\boldsymbol{x_{j, t}}, \boldsymbol{y_{i, t}}) + \boldsymbol{n_{i, j, t}},\\
% h(\boldsymbol{x_{j, t}}, \boldsymbol{y_{i, t}})
% &:=\left[\begin{array}{c}
% r_{i, j, t} \\
% \alpha_{i, j, t}
% \end{array}\right]\\
% &:=\left[\begin{array}{c}
% \sqrt{\left(y_{i, t}^1-x_{j, t}^1\right)^2+\left(y_{i, t}^2-x_{j, t}^2\right)^2} \\
% \arctan \left(\left(y_{i, t}^2-x_{j, t}^2\right)\left(y_{i, t}^1-x_{j, t}^1\right)\right)-\phi
% \end{array}\right]\\
% \boldsymbol{n_{i, j, t}}
% &:= [n_{i, j, t}^r, n_{i, j, t}^\alpha]^T
% \end{aligned},\\
% \text{$n_{i, j, t}^r$ is drawn from $p(n^r)$}, \\
% \text{$n_{i, j, t}^\alpha$ is drawn from $p(n^\alpha)$}.
% \end{gathered}
% \label{z}
% \end{equation}
% The noise models for range and bearing measurements are denoted as $p(n^r)$ and $p(n^\alpha)$, respectively, and are empirically obtained from our testbed.
% $p(n^r)$ and $p(n^\alpha)$ are specified as a normal distribution with mean $\mu = 0$ and variance $\sigma$, expressed as a percentage of $r_{i, j, t}$ and $\alpha_{i, j, t}$.
% % For bearing measurements, $p(n^\alpha)$ is also specified as a normal distribution with mean $\mu = 0$ and a constant variance, as the bearing measurement noise does not depend on the bearing between $A_j$ and $B_i$, as shown in \cite{kalaitzakis2021fiducial}.

% \subsection{Linearization of Observation model} 
% % To linearize the observation model of AMAV,
% % We utilize the mean of BMAV's location estimation for linearization. 
% % For a Gaussian distribution, the mean of BMAV's location estimation is the most probable location. 
% We compute the Jacobian matrix of $h(\boldsymbol{x}, \boldsymbol{y})$ based on Taylor expansion by taking the gradient with respect to the location estimation of $\boldsymbol{y}$ to linearize the observation model,

% \begin{equation}
% % \vspace{-0.5em}
% \setlength\abovedisplayskip{3pt}%shrink space
% \setlength\belowdisplayskip{3pt}
% \begin{aligned}
% &\nabla_{\boldsymbol{y}} h(\boldsymbol{x}, \boldsymbol{y})\\
% &=\frac{1}{r(\boldsymbol{x}, \boldsymbol{y})}\left[\begin{array}{cc}
% \left(y^1-x^1\right) & \left(y^2-x^2\right) \\
% -\sin \left(\phi+\alpha(\boldsymbol{x}, \boldsymbol{y})\right) & \cos \left(\phi+\alpha(\boldsymbol{x}, \boldsymbol{y})\right)
% \end{array}\right].
% \end{aligned}
% \label{linearize}
% % \vspace{-0.4em}
% \end{equation}
% % where $h$ is the observation model of AMAV and $\boldsymbol{x}$ is the state of AMAV.



% To simplify notation, we let
% % \boldsymbol{B} := [B_1, \dots, B_N]\boldsymbol{B} := [B_1, \dots, B_N], 
% % \boldsymbol{A} := [A_1, \dots, A_M]\boldsymbol{A} := [A_1, \dots, A_M], 
% $\boldsymbol{y_t} := {[\boldsymbol{y_{1, t}^T}, \dots, \boldsymbol{y_{N, t}^T}]}^T$, 
% % \boldsymbol{v_t} := {[\boldsymbol{v_{1, t}^T}, \dots, \boldsymbol{v_{N, t}^T}]}^T\boldsymbol{v_t} := {[\boldsymbol{v_{1, t}^T}, \dots, \boldsymbol{v_{N, t}^T}]}^T, 
% % \boldsymbol{\dot{v}_t} := {[\boldsymbol{\dot{v}_{1, t}^T}, \dots, \boldsymbol{\dot{v}_{N, t}^T}]}^T\boldsymbol{\dot{v}_t} := {[\boldsymbol{\dot{v}_{1, t}^T}, \dots, \boldsymbol{\dot{v}_{N, t}^T}]}^T, 
% $\boldsymbol{x_t} := {[\boldsymbol{x_{1, t}^T}, \dots, \boldsymbol{x_{M, t}^T}]}^T$, 
% $\boldsymbol{u_t} := {[\boldsymbol{u_{1, t}^T}, \dots, \boldsymbol{u_{M, t}^T}]}^T$, 
% % % \boldsymbol{z_{j, t}} := {[\boldsymbol{z_{1, j, t}^T}, \dots, \boldsymbol{z_{N, j, t}^T}]}^T\boldsymbol{z_{j, t}} := {[\boldsymbol{z_{1, j, t}^T}, \dots, \boldsymbol{z_{N, j, t}^T}]}^T, 
% $\boldsymbol{\widehat{y}_t} := {[\boldsymbol{\widehat{y}_{1, t}^T}, \dots, \boldsymbol{\widehat{y}_{N, t}^T}]}^T$, 
% % % \boldsymbol{y_t}^{-} := {[\boldsymbol{y_{1, t}^T}^{-}, \dots, \boldsymbol{y_{N, t}^T}^{-}]}^T\boldsymbol{y_t}^{-} := {[\boldsymbol{y_{1, t}^T}^{-}, \dots, \boldsymbol{y_{N, t}^T}^{-}]}^T, 
% % % \boldsymbol{y_t}^{+} := {[\boldsymbol{y_{1, t}^T}^{+}, \dots, \boldsymbol{y_{N, t}^T}^{+}]}^T\boldsymbol{y_t}^{+} := {[\boldsymbol{y_{1, t}^T}^{+}, \dots, \boldsymbol{y_{N, t}^T}^{+}]}^T, 
% ${\Sigma_{t}} := {diag(\Sigma_{1, t}^T, \dots, \Sigma_{N, t}^T)}^T$. 
% % % {\Sigma_{t}}^+ := {[{\Sigma_{1, t}^T}^+, \dots, {\Sigma_{N, t}^T}^+]}^T{\Sigma_{t}}^+ := {[{\Sigma_{1, t}^T}^+, \dots, {\Sigma_{N, t}^T}^+]}^T, 
% % % {\Sigma_{t}}^- := {[{\Sigma_{1, t}^T}^-, \dots, {\Sigma_{N, t}^T}^-]}^T{\Sigma_{t}}^- := {[{\Sigma_{1, t}^T}^-, \dots, {\Sigma_{N, t}^T}^-]}^T,
% % \chi := \chi_1 * \dots * \chi_M\chi := \chi_1 * \dots * \chi_M, and U := U_1 * \dots * U_MU := U_1 * \dots * U_M.

% % \section{MSE of an estimator} \label{MSE}\
% % The location of BAMVs is $\boldsymbol{y_t}$, and the estimation is $\boldsymbol{\hat{y}_t}$.
% % \begin{equation}
% % \begin{aligned}
% % & \mathrm{E}\left[\|\boldsymbol{\hat{y}_{1:t}}-\boldsymbol{y_{1:t}}\|^2\right] = \operatorname{MSE}(\boldsymbol{\hat{y}_{1:t}})\\
% % & =\mathrm{E}\left[\sum(\boldsymbol{\hat{y}_{1:t}}-\mathrm{E}[\boldsymbol{\hat{y}_{1:t}}])^2\right]+\operatorname{Bias}[\boldsymbol{\hat{y}_{1:t}}]^{\top} \operatorname{Bias}[\boldsymbol{\hat{y}_{1:t}}] \\
% % & = \operatorname{tr}(\Sigma_t) + (\|\operatorname{Bias}[\boldsymbol{\hat{y}_t}]\|)^2.
% % &
% % \end{aligned}
% % \end{equation}
% % % Although the observation generated by AMAVs for BMAVs is nonlinear, 
% % The estimator of BMAVs' location is unbiased after linearization of observation, which means $\|\operatorname{Bias}[\boldsymbol{\hat{y}_t}]\| = 0$.
% % Therefore, $\operatorname{MSE}(\boldsymbol{\hat{y}_{1:t}}) = \operatorname{tr}(\Sigma_t)$.


% \section{Problem Formulation}\label{A2}
% % \subsection{Optimized Objective}
% % The goal of H-Swarm is to allocate the sensing resources of AMAVs to limit the localization error of BMAVs.
% % Specifically, given a finite time horizon $T$, we select a sequence of motion commands of AMAVs $\boldsymbol{u_{0:T-1}}$, to limit the localization error of BMAVs in $T$.
% % The localization error of BMAVs can be mathematically expressed as 
% % % \begin{equation}
% % % \psi(T) := \sum_{t=1}^T\left(E\left[{||\boldsymbol{y_t}-\boldsymbol{\widehat{y}_t}||}^2\right]\right),
% % % \label{le}
% % % \end{equation}
% % $\psi(T) := \sum_{t=1}^T(E[{||\boldsymbol{y_t}- \boldsymbol{\widehat{y}_t}||}^2])$.
% % % which is the sum of mean squared error (MSE) of $\boldsymbol{\widehat{y}_t}$.
% % However, to compute $\psi$, we require the actual locations of BMAVs, which are not obtainable due to their limited abilities and the absence of external localization infrastructure.
% % As a result, minimizing $\psi$ cannot guide the sensing resources allocation of AMAVs. 
% % Instead, we opt to optimize a measure of information reflecting the quality of BMAVs' location estimations.
% % Specifically, we choose to optimize the trace of the covariance matrix of BMAVs' location estimations \cite{ucinski2004optimal}, which can be mathematically expressed as 
% % % \begin{equation}
% % % \xi(T) := \sum_{t=1}^T\left(tr\left(\Sigma_t\right)\right).
% % % \label{ob}
% % % \end{equation}
% % $\xi(T) := \sum_{t=1}^T(tr(\Sigma_t)).$
% % This objective measures the uncertainty of location estimations, a lower value indicates greater certainty and vice versa.

% % \subsection{Problem Formulation}

% We aim to optimize the trace of the covariance of BMAVs’ location estimation $\Sigma_t$ to limit the localization error within a finite time horizon $T$, considering the motion commands of each AMAV within $T$.
% The mathematically formulated sensing resource allocation problem is given by,
% \begin{equation}
% \min _{\boldsymbol{u_0}, \ldots, \boldsymbol{u_{T-1}}} \xi(T) = \sum_{t=1}^T\left(tr\left(\Sigma_t\right)\right),
% \end{equation}
% \text {\centerline{s.t.} }
% \begin{align}
%     & \boldsymbol{x_{t+1}} = f(\boldsymbol{x_{t}}, \boldsymbol{u_{t}}), t \in \{0,\dots, T-1\} \\
%     & 0 \leq x_{j, t}^1, y_{i, t}^1 \leq L, \\
%     & \quad j \in \{0,\dots, N\}, i \in \{0,\dots, M\}, t\in\{0,\dots, T-1\} \notag \\
%     & 0 \leq x_{j, t}^2, y_{i, t}^2 \leq W, \\
%     & \quad j \in \{0,\dots, N\}, i \in \{0,\dots, M\}, t\in\{0,\dots, T-1\} \notag \\
%     & \Sigma_{t+1}=\rho_{t+1}^e\left(\rho_t^p\left(\Sigma_t\right), \boldsymbol{x}_{t+1}\right), t\in\{0,\dots, T-1\}.
% \label{problem}
% \end{align}
% $\rho_t^e$ and $\rho_{t+1}^p$ are correction and prediction steps, which are described in Section III-B.


% \section{MSE of an estimator} \label{MSE}\
% The location of BAMVs is $\boldsymbol{y_t}$, and the estimation is $\boldsymbol{\hat{y}_t}$.
% \begin{equation}
% \begin{aligned}
% & \mathrm{E}[\|\boldsymbol{\hat{y}_t}-\boldsymbol{y_t}\|^2] = \operatorname{MSE}(\boldsymbol{\hat{y}_t})\\
% % & =E[(\sqrt{(\boldsymbol{\hat{y}_t}-\boldsymbol{y_t})^{\top}(\boldsymbol{\hat{y}_t}-\boldsymbol{y_t})})^2] \\
% % & =E[(\boldsymbol{\hat{y}_t}-\boldsymbol{y_t})^{\top}(\boldsymbol{\hat{y}_t}-\boldsymbol{y_t})] \\
% % & =\mathrm{E}[(\boldsymbol{\hat{y}_t}-\mathrm{E}[\boldsymbol{\hat{y}_t}]+\mathrm{E}[\boldsymbol{\hat{y}_t}]-\boldsymbol{y_t})^{\top}(\widehat{\boldsymbol{y_t}}-\mathrm{E}[\boldsymbol{\hat{y}_t}]+\mathrm{E}[\boldsymbol{\hat{y}_t}]-\boldsymbol{y_t})] \\
% & =\mathrm{E}[(\boldsymbol{\hat{y}_t}-\mathrm{E}[\boldsymbol{\hat{y}_t}])^{\top}(\boldsymbol{\hat{y}_t}-\mathrm{E}[\boldsymbol{\hat{y}_t}])+(\boldsymbol{\hat{y}_t}-\mathrm{E}[\boldsymbol{\hat{y}_t}])^{\top}(\mathrm{E}[\boldsymbol{\hat{y}_t}]-\boldsymbol{y_t}) \\
% & \quad +(\mathrm{E}[\boldsymbol{\hat{y}_t}]-\boldsymbol{y_t})^{\top}(\boldsymbol{\hat{y}_t}-\mathrm{E}[\boldsymbol{\hat{y}_t}])+(\mathrm{E}[\boldsymbol{\hat{y}_t}]-\boldsymbol{y_t})^{\top}(\mathrm{E}[\boldsymbol{\hat{y}_t}]-\boldsymbol{y_t})] \\
% & =\mathrm{E}[(\boldsymbol{\hat{y}_t}-\mathrm{E}[\boldsymbol{\hat{y}_t}])^{\top}(\boldsymbol{\hat{y}_t}-\mathrm{E}[\boldsymbol{\hat{y}_t}])]+\mathrm{E}[(\boldsymbol{\hat{y}_t}-\mathrm{E}[\boldsymbol{\hat{y}_t}])^{\top}(\mathrm{E}[\boldsymbol{\hat{y}_t}]-\boldsymbol{y_t})] \\
% & \quad +\mathrm{E}[(\mathrm{E}[\boldsymbol{\hat{y}_t}]-\boldsymbol{y_t})^{\top}(\boldsymbol{\hat{y}_t}-\mathrm{E}[\boldsymbol{\hat{y}_t}])]+\mathrm{E}[(\mathrm{E}[\boldsymbol{\hat{y}_t}]-\boldsymbol{y_t})^{\top}(\mathrm{E}[\boldsymbol{\hat{y}_t}]-\boldsymbol{y_t})] \\
% & \quad +(\mathrm{E}[\boldsymbol{\hat{y}_t}]-\boldsymbol{y_t})^{\top} \cdot 0+(\mathrm{E}[\boldsymbol{\hat{y}_t}]-\boldsymbol{y_t})^{\top}(\mathrm{E}[\boldsymbol{\hat{y}_t}]-\boldsymbol{y_t}) \\
% & =\mathrm{E}[(\boldsymbol{\hat{y}_t}-\mathrm{E}[\boldsymbol{\hat{y}_t}])^{\top}(\boldsymbol{\hat{y}_t}-\mathrm{E}[\boldsymbol{\hat{y}_t}])]+(\mathrm{E}[\boldsymbol{\hat{y}_t}]-\boldsymbol{y_t})^{\top}(\mathrm{E}[\boldsymbol{\hat{y}_t}]-\boldsymbol{y_t}) \\
% & =\mathrm{E}[\sum(\boldsymbol{\hat{y}_t}-\mathrm{E}[\boldsymbol{\hat{y}_t}])^2]+\operatorname{Bias}[\boldsymbol{\hat{y}_t}]^{\top} \operatorname{Bias}[\boldsymbol{\hat{y}_t}] \\
% &= \operatorname{tr}(\Sigma_t) + (\|\operatorname{Bias}[\boldsymbol{\hat{y}_t}]\|)^2.
% &
% \end{aligned}
% \end{equation}

% Although the observation generated by AMAVs for BMAVs is nonlinear, the estimator of BMAVs' location is unbiased after linearization of observation, which means $\|\operatorname{Bias}[\boldsymbol{\hat{y}_t}]\| = 0$.
% Therefore, $\operatorname{MSE}(\boldsymbol{\hat{y}_t}) = \operatorname{tr}(\Sigma_t)$.

% \section{Main notations and description}\label{notation}
% The main symbols are as follows:
% \begin{table}[h]
%     % \centering
%     % \caption{Main notations and Descriptions}

%     \begin{tabular}{ll}
%        \toprule
%        \textbf{Notation}                & \textbf{Description} \\
%        \midrule
%        \textbf{Environment}\\
%         $\Omega$                       & The environment MAV swarm operates in.\\
%         $B_i, \boldsymbol{B}$            & The $i$-th BMAV and set of BMAVs.\\
%         $A_j, \boldsymbol{A}$            & The $j$-th AMAV and set of AMAVs.\\
%         \midrule
%         \textbf{State model of BMAV}\\
%         $\delta$            &Time interval between two commands. \\
%         $\boldsymbol{y_{i, t}}$        & Location of $B_i$.\\
%         $\boldsymbol{v_{i, t}}, \boldsymbol{\dot{v}_{i, t}}$    & Motion command and motion measurement.\\
%         % $$    & Motion measurement of $B_i$.\\
%         $n_{i, t}^1, n_{i, t}^2, p(n^1), p(n^2)$    &The motion noise and motion noise model .\\
%         $\boldsymbol{\widehat{y}_{i, t}}, \boldsymbol{{y_{i, t}}^{-}}, \boldsymbol{{y_{i, t}}^{+}}$    & Location estimation of $B_i$.\\
%         % $$    & The prior of $B_i$'s location estimation.\\
%         % $$    & The posterior of $B_i$'s location estimation.\\
%         % ${\Sigma_{i, t}}, {\Sigma_{i, t}}^+, {\Sigma_{i, t}}^-$    & Covariance matrix of $B_i$'s location estimation maintained by system.\\
%         ${\Sigma_{i, t}}, {\Sigma_{i, t}}^+, {\Sigma_{i, t}}^-$    & Covariance matrix of $B_i$'s location estimation.\\
%         % ${\Sigma_{j, t}}$  & Covariance matrix maintained by $A_j$ when planning.\\
%         ${\Sigma_{j, t}}$  & Covariance matrix maintained by $A_j$.\\
%         \midrule
%         \textbf{State model of AMAV}\\
%         $\boldsymbol{x_{j, t}}$    &Location of $A_j$.\\
%         % $\chi_j$    & State set of $A_j$.\\
%         $d_{\chi}$   & Distance between two AMAVs' locations.\\
%         $\boldsymbol{u_{j, t}}, u_{j,t}, \omega_{j,t}$    & Velocity command of $A_j$.\\
%         % $$                &  Translational velocity of $A_j$.\\
%         % $$            & Rotational velocity of $A_j$.\\
%         % $U_j$                        & Set of velocity commands of $A_j$.\\
%         \midrule
%         \textbf{Observation model}\\
%         $F_{j, t}$                    & Field of view (FoV) of $A_j$.\\
%         $\theta$                    & Observation angle of the visual sensor.\\
%         $r_m$                        & The longest distance to generate observation.\\
%         $z_{i, j, t}$                & The observation for $B_i$ generated by $A_j$.\\
%         $r_{i, j, t}, \alpha_{i, j, t}$            & The range and bearing between $A_j$ and $B_i$.\\
%         % $$            & The bearing between $A_j$ and $B_i$.\\
%         $n_{i, j, t}^r, n_{i, j, t}^\alpha$                & Range and bearing measurement noise. \\
%         % $$             & The noise of bearing measurement. \\
%         $p(n^r), p(n^\alpha)$                        & Range and bearing measurement noise model. \\
%         % $$                    & Noise model of bearing measurement. \\
        

%         % $\boldsymbol{y_t}$           & Set of BMAVs' locations at time $t$.\\
%         % $\boldsymbol{v_t}$           & Set of BMAVs' velocity commands at time $t$.\\
%         % $\boldsymbol{\dot{v}_t}$           & Set of BMAVs' velocity measurements at time $t$.\\
%         % $\boldsymbol{\widehat{y}_t}$    & Set of BMAVs' location estimations at time $t$.\\
%         % $\boldsymbol{x_{t}}$            & Set of AMAVs' location at time $t$. \\
%        \bottomrule
%     \end{tabular}
% \label{notation}
% \end{table}
